# Supplementary material for: RRNet: Towards ReLU-Reduced Neural Network for Two-party Computation Based Private Inference
Source: arXiv:2302.02292 source file (2023-02-22)
Supplement: Supplementary file 1 [file Appendix_convergence.tex]

\section{Convergence Prove of $X^2act$}
\label{sec:x2act_conv}
In this section, we study convergence of $X^2act$ neural network convergence problem. we define input $x \in [0,1]^{m\times n}$, the output of the network is $f(x) \in \mathbb{R}$. We consider k-th layer with the activation function $\sigma$ defined in Eq.~\ref{eq:x2act}, and it can be represented as:
\begin{equation}
f_k(x)= \sigma({\bf{W}}^kx_{k} +{\bf{b}}^k)
\end{equation}
For n layers network, it can be represented as:
\begin{equation}
    f(x)=f_n \cdot f_{n-1} \cdot f_{n-2} \cdot ...\cdot f_1
\end{equation}
{\bf{Theorem 1}} Let $x \in \Omega\subseteq R^d$, where $\Omega$ is Lebesgue measurable set. $f = f_n \cdot f_{n-1} \cdot f_{n-2} \cdot ...\cdot f_1$ is the $X^2act$ function,  $g= g_n \cdot g_{n-1} \cdot g_{n-2} \cdot ...\cdot g_1$ is the function of with the activation domain $D_{m_k}$ from f, where $m_k$ depend on the dimension of each layer. So that if
\begin{equation}
\lim_{n\rightarrow \infty }\sum_{k=1}^{n} \int_{D_{m_k}}\left \| g_k(x)-f_k(x) \right \|^p_pdx=0
\end{equation}
and 
where $\left \| \cdot \right \|_p$ is the $l^p$ norm,
then $f$ converge to $g$, such that:
\begin{equation}
    \lim_{n\rightarrow \infty }\left \| f-g \right \|=0
\end{equation}
Theorem 1 is proved in \cite{dasgupta1992power}. 

Then we use Theorem 1 to show the suitable of $X^2act$.
For each layer of network, the output can be rewritten as:
\begin{equation}
    \begin{aligned}
        &f_k(x)= \sigma({\bf{W}}^kx_{k} +{\bf{b}}^k)=\frac{c}{\sqrt[]{N_x}} w_1 x^2 + w_2 x + b =
        \\ &\frac{c}{\sqrt[]{N_x}}w_1(x+\frac{w_2}{2w_1}\frac{\sqrt{N_x}}{c})^2-\frac{\sqrt[]{N_x}}{c} \cdot \frac{w_2^2}{w_1}+b \geq -\frac{\sqrt[]{N_x}}{c} \cdot \frac{w_2^2}{w_1}+b
    \end{aligned}
\end{equation}
So that there is an activation domain  $D^f_{m_k}$, such that:
\begin{equation}
    D_{m_k}^f=\{ x \in \mathbb{R}^{m_k}: f_k\geq -\frac{\sqrt[]{N_x}}{c} \cdot \frac{w_2^2}{w_1}+b, where f = f_n \cdot f_{n-1} \cdot f_{n-2} \cdot ...\cdot f_1 \}
\end{equation} and $f$ with the limit value $-\frac{\sqrt[]{N_x}}{c} \cdot \frac{w_2^2}{w_1}+b$.
According to \cite{xu2021convergence}, there \textbf{exist} a subset of $D_{m_k} \subseteq D_{m_k}^f$, which satisfied the condition 
\begin{equation}
\lim_{n\rightarrow \infty }\sum_{k=1}^{n} \int_{D_{m_k}}\left \| g_k(x)-f_k(x) \right \|^p_pdx=0
\end{equation} where $p < \infty$.
